# Supplementary material for: Learned Low Precision Graph Neural Networks
Source: arXiv:2009.09232 source file (2020-09-19)
Supplement: Supplementary file 1 [file supp.tex]

\documentclass{article}

% if you need to pass options to natbib, use, e.g.:
\PassOptionsToPackage{numbers, compress}{natbib}
% before loading neurips_2020

% ready for submission
\usepackage{neurips_2020}

% to compile a preprint version, e.g., for submission to arXiv, add add the
% [preprint] option:
% \usepackage[preprint]{neurips_2020}
% to compile a camera-ready version, add the [final] option, e.g.:
% \usepackage[final]{neurips_2020}

% to avoid loading the natbib package, add option nonatbib:
%  \usepackage[nonatbib]{neurips_2020}

\usepackage[utf8]{inputenc} % allow utf-8 input
\usepackage[T1]{fontenc}    % use 8-bit T1 fonts
\usepackage{hyperref}       % hyperlinks
\usepackage{url}            % simple URL typesetting
\usepackage{booktabs}       % professional-quality tables
\usepackage{amsfonts}       % blackboard math symbols
\usepackage{nicefrac}       % compact symbols for 1/2, etc.
\usepackage{microtype}      % microtypography
\usepackage{multirow}
\usepackage[table]{xcolor}
\usepackage{natbib}
\usepackage{adjustbox}

\usepackage{algorithm2e,algorithmic}
\usepackage{amsmath,amsfonts}
\usepackage{cleveref}

\DeclareMathOperator*{\argmax}{arg\,max}
\DeclareMathOperator*{\argmin}{arg\,min}
\newcommand{\eg}{\textit{e.g\@.}}
\newcommand{\etc}{\textit{etc.}}
\newcommand{\etal}{\textit{et~al\@.}}
\newcommand{\ie}{\textit{i.e\@.}}
\newcommand{\vs}{\textit{vs\@.}}

\title{Appendix for Learned Low Precision Graph Neural Networks}

% The \author macro works with any number of authors. There are two commands
% used to separate the names and addresses of multiple authors: \And and \AND.
%
% Using \And between authors leaves it to LaTeX to determine where to break the
% lines. Using \AND forces a line break at that point. So, if LaTeX puts 3 of 4
% authors names on the first line, and the last on the second line, try using
% \AND instead of \And before the third author name.

\author{%
  Yiren Zhao\thanks{Equal contribution. Correspondence to Yiren Zhao (yiren.zhao@cl.cam.ac.uk).} \And
  Duo Wang\footnotemark[1] \And
  Daniel Bates \And
  Robert Mullins  \And
  Mateja Jamnik  \And
  Pietro Lio
  \And
  Department of Compute Science and Technology, University of Cambridge \\
  Cambridge, UK, CB3 0FD \\
  % \texttt{yiren.zhao@cl.cam.ac.uk}
  % Coauthor \\
  % Affiliation \\
  % Address \\
  % \texttt{email} \\
  % \And
  % Coauthor \\
  % Affiliation \\
  % Address \\
  % \texttt{email} \\
  % \And
  % Coauthor \\
  % Affiliation \\
  % Address \\
  % \texttt{email} \\
}

\begin{document}

\maketitle
\input{sections/appendix.tex}
\bibliographystyle{abbrvnat}
\bibliography{references}


\end{document}
